# Supplementary material for: Pathfinding Neural Cellular Automata
Source: arXiv:2301.06820 source file (2023-01-17)
Supplement: Supplementary file 1 [file diameter_cut_corners_cross_eval_selective.tex]

\begin{tabular}{|c|r|r|r|r|r|r|r|}
\hline
    &      &    &      model &                  train & \multicolumn{3}{c|}{test} \\
\cline{4-8}
\cline{4-8}
    &      &    &        --- &                  16x16 &                  16x16 & \multicolumn{2}{c|}{32x32} \\
\cline{4-8}
\cline{4-8}
    &      &    &  n. params &          pct. complete &          pct. complete &             accuracies &         pct. complete \\
\textbf{model} & \textbf{cut corners} & \textbf{n. hid chan} &            &                        &                        &                        &                       \\
\hline
\multirow{4}{*}{\textbf{NCA}} & \multirow{2}{*}{\textbf{False}} & \textbf{48} &  1,382,400 &           98.64 ± 0.83 &           46.19 ± 3.23 &          -0.58 ± 17.41 &           1.14 ± 0.54 \\
    &      & \textbf{96} &  5,419,008 &  \textbf{99.45} ± 0.17 &  \textbf{58.65} ± 2.32 &  \textbf{21.31} ± 3.46 &  \textbf{3.80} ± 0.97 \\
\cline{2-8}
    & \multirow{2}{*}{\textbf{True}} & \textbf{48} &    768,000 &          58.00 ± 52.95 &          33.81 ± 30.92 &            4.43 ± 5.10 &           1.15 ± 1.08 \\
    &      & \textbf{96} &  3,010,560 &           99.16 ± 0.22 &           55.56 ± 1.72 &           10.16 ± 5.86 &           1.51 ± 0.46 \\
\hline
\end{tabular}
