# Supplementary material for: Pathfinding Neural Cellular Automata
Source: arXiv:2301.06820 source file (2023-01-17)
Supplement: Supplementary file 2 [file diameter_evo_data_cross_eval_selective.tex]

\begin{tabular}{|c|r|r|r|r|r|r|r|r|}
\hline
    &      &    &      model &                  train & \multicolumn{4}{c|}{test} \\
\cline{4-9}
\cline{4-9}
    &      &    &        --- &                  16x16 & \multicolumn{2}{c|}{16x16} & \multicolumn{2}{c|}{32x32} \\
\cline{4-9}
\cline{4-9}
    &      &    &  n. params &          pct. complete &             accuracies &          pct. complete &             accuracies &          pct. complete \\
\textbf{model} & \textbf{env generation} & \textbf{n. hid chan} &            &                        &                        &                        &                        &                        \\
\hline
\multirow{4}{*}{\textbf{NCA}} & \multirow{2}{*}{\textbf{False}} & \textbf{48} &  1,382,400 &           98.64 ± 0.83 &           72.54 ± 4.27 &           46.19 ± 3.23 &          -0.58 ± 17.41 &            1.14 ± 0.54 \\
    &      & \textbf{96} &  5,419,008 &  \textbf{99.45} ± 0.17 &           78.51 ± 1.04 &           58.65 ± 2.32 &           21.31 ± 3.46 &            3.80 ± 0.97 \\
\cline{2-9}
    & \multirow{2}{*}{\textbf{True}} & \textbf{48} &  1,382,400 &          65.90 ± 17.29 &           83.81 ± 5.05 &          61.16 ± 10.40 &          30.00 ± 11.45 &            5.26 ± 2.71 \\
    &      & \textbf{96} &  5,419,008 &           72.22 ± 1.96 &  \textbf{87.90} ± 0.94 &  \textbf{74.23} ± 1.26 &  \textbf{40.68} ± 4.31 &  \textbf{10.39} ± 1.20 \\
\hline
\end{tabular}
