# Supplementary material for: Pathfinding Neural Cellular Automata
Source: arXiv:2301.06820 source file (2023-01-17)
Supplement: Supplementary file 3 [file diameter_kernel_cross_eval_selective.tex]

\begin{tabular}{|c|r|r|r|r|r|r|r|r|}
\hline
    &   &       &    &       model &                  train & \multicolumn{3}{c|}{test} \\
\cline{5-9}
\cline{5-9}
    &   &       &    &         --- &                  16x16 &                  16x16 & \multicolumn{2}{c|}{32x32} \\
\cline{5-9}
\cline{5-9}
    &   &       &    &   n. params &          pct. complete &          pct. complete &             accuracies &         pct. complete \\
\textbf{model} & \textbf{kernel size} & \textbf{max pool} & \textbf{n. hid chan} &             &                        &                        &                        &                       \\
\hline
\multirow{4}{*}{\textbf{NCA}} & \multirow{2}{*}{\textbf{3}} & \multirow{2}{*}{\textbf{False}} & \textbf{48} &   1,382,400 &           98.64 ± 0.83 &           46.19 ± 3.23 &          -0.58 ± 17.41 &           1.14 ± 0.54 \\
    &   &       & \textbf{96} &   5,419,008 &           99.45 ± 0.17 &  \textbf{58.65} ± 2.32 &  \textbf{21.31} ± 3.46 &  \textbf{3.80} ± 0.97 \\
\cline{2-9}
\cline{3-9}
    & \multirow{2}{*}{\textbf{5}} & \multirow{2}{*}{\textbf{False}} & \textbf{48} &   3,840,000 &           99.54 ± 0.08 &           36.43 ± 2.43 &          -23.37 ± 6.61 &           0.52 ± 0.24 \\
    &   &       & \textbf{96} &  15,052,800 &  \textbf{99.60} ± 0.14 &           46.36 ± 2.18 &           0.09 ± 10.06 &           2.23 ± 0.74 \\
\hline
\end{tabular}
