# Supplementary material for: Pathfinding Neural Cellular Automata
Source: arXiv:2301.06820 source file (2023-01-17)
Supplement: Supplementary file 4 [file diameter_max_pool_cross_eval_selective.tex]

\begin{tabular}{|c|r|r|r|r|r|r|r|}
\hline
    &      &     &      model &                  train & \multicolumn{3}{c|}{test} \\
\cline{4-8}
\cline{4-8}
    &      &     &        --- &                  16x16 &                  16x16 & \multicolumn{2}{c|}{32x32} \\
\cline{4-8}
\cline{4-8}
    &      &     &  n. params &          pct. complete &          pct. complete &              accuracies &          pct. complete \\
\textbf{model} & \textbf{max pool} & \textbf{n. hid chan} &            &                        &                        &                         &                        \\
\hline
\multirow{6}{*}{\textbf{NCA}} & \multirow{3}{*}{\textbf{False}} & \textbf{48 } &  1,382,400 &           98.64 ± 0.83 &           46.19 ± 3.23 &           -0.58 ± 17.41 &            1.14 ± 0.54 \\
    &      & \textbf{96 } &  5,419,008 &  \textbf{99.45} ± 0.17 &  \textbf{58.65} ± 2.32 &            21.31 ± 3.46 &            3.80 ± 0.97 \\
    &      & \textbf{128} &  9,584,640 &           99.30 ± 0.33 &           58.50 ± 3.66 &            20.80 ± 5.11 &            4.16 ± 1.35 \\
\cline{2-8}
    & \multirow{3}{*}{\textbf{True}} & \textbf{48 } &  1,382,400 &          78.41 ± 43.83 &          37.00 ± 21.22 &           -5.62 ± 29.69 &            3.96 ± 4.22 \\
    &      & \textbf{96 } &  5,419,008 &           98.91 ± 0.45 &           53.49 ± 4.89 &           17.97 ± 23.83 &            9.79 ± 5.82 \\
    &      & \textbf{128} &  9,584,640 &           99.24 ± 0.25 &           53.66 ± 8.45 &  \textbf{22.90} ± 32.36 &  \textbf{11.54} ± 7.32 \\
\hline
\end{tabular}
