# Supplementary material for: Pathfinding Neural Cellular Automata
Source: arXiv:2301.06820 source file (2023-01-17)
Supplement: Supplementary file 5 [file diameter_max_pool_cross_eval_selective_many1.tex]

\begin{tabular}{|c|r|r|r|r|r|r|r|}
\hline
    &      &     &     model &                  train & \multicolumn{3}{c|}{test} \\
\cline{4-8}
\cline{4-8}
    &      &     &       --- &                  16x16 &                  16x16 & \multicolumn{2}{c|}{32x32} \\
\cline{4-8}
\cline{4-8}
    &      &     & n. params &          pct. complete &          pct. complete &             accuracies &          pct. complete \\
\textbf{model} & \textbf{max pool} & \textbf{n. hid chan} &           &                        &                        &                        &                        \\
\hline
\multirow{10}{*}{\textbf{NCA}} & \multirow{5}{*}{\textbf{False}} & \textbf{48 } &    21,600 &           50.28 ± 5.68 &           43.54 ± 5.31 &            9.68 ± 7.11 &            1.44 ± 1.46 \\
    &      & \textbf{64 } &    38,016 &           66.50 ± 5.21 &           53.85 ± 6.30 &           28.14 ± 6.04 &            7.42 ± 2.96 \\
    &      & \textbf{96 } &    84,672 &           90.93 ± 3.77 &           64.39 ± 6.38 &           25.65 ± 8.14 &           15.73 ± 4.01 \\
    &      & \textbf{128} &   149,760 &  \textbf{94.08} ± 2.67 &           68.41 ± 5.70 &         -96.77 ± 18.97 &            7.14 ± 3.26 \\
    &      & \textbf{150} &   205,200 &           86.00 ± 4.40 &           68.60 ± 5.80 &           23.30 ± 7.18 &            9.94 ± 4.12 \\
\cline{2-8}
    & \multirow{5}{*}{\textbf{True}} & \textbf{48 } &    21,600 &           40.23 ± 5.64 &           35.03 ± 5.92 &          -18.73 ± 7.24 &            0.13 ± 0.48 \\
    &      & \textbf{64 } &    38,016 &           61.12 ± 6.26 &           49.65 ± 6.06 &          -44.44 ± 8.51 &            0.01 ± 0.14 \\
    &      & \textbf{96 } &    84,672 &           82.96 ± 4.56 &           66.55 ± 6.14 &  \textbf{69.80} ± 5.71 &  \textbf{48.05} ± 6.32 \\
    &      & \textbf{128} &   149,760 &           89.99 ± 4.01 &           70.10 ± 6.39 &           64.12 ± 6.29 &           45.19 ± 5.85 \\
    &      & \textbf{150} &   205,200 &           91.58 ± 3.43 &  \textbf{70.64} ± 5.96 &           64.40 ± 6.40 &           48.03 ± 7.10 \\
\hline
\end{tabular}
