# Supplementary material for: Pathfinding Neural Cellular Automata
Source: arXiv:2301.06820 source file (2023-01-17)
Supplement: Supplementary file 6 [file diameter_models_cross_eval_selective.tex]

\begin{tabular}{|c|r|r|r|r|r|r|r|}
\hline
    &    &     &       model &                  train & \multicolumn{3}{c|}{test} \\
\cline{4-8}
\cline{4-8}
    &    &     &         --- &                  16x16 & \multicolumn{2}{c|}{16x16} &                 32x32 \\
\cline{4-8}
\cline{4-8}
    &    &     &   n. params &          pct. complete &             accuracies &          pct. complete &         pct. complete \\
\textbf{model} & \textbf{n layers} & \textbf{n. hid chan} &             &                        &                        &                        &                       \\
\hline
\multirow{3}{*}{\textbf{GCN}} & \multirow{3}{*}{\textbf{16}} & \textbf{96 } &       9,408 &            0.00 ± 0.00 &            4.13 ± 8.95 &            0.00 ± 0.00 &           0.00 ± 0.00 \\
    &    & \textbf{128} &      16,640 &            0.00 ± 0.00 &           8.66 ± 11.86 &            0.00 ± 0.00 &           0.00 ± 0.00 \\
    &    & \textbf{256} &      66,048 &            0.00 ± 0.00 &           8.72 ± 11.95 &            0.00 ± 0.00 &           0.00 ± 0.00 \\
\cline{1-8}
\cline{2-8}
\multirow{3}{*}{\textbf{MLP}} & \multirow{3}{*}{\textbf{16}} & \textbf{96 } &  16,091,136 &           24.46 ± 8.83 &           -8.08 ± 2.47 &            0.00 ± 0.00 &           0.00 ± 0.00 \\
    &    & \textbf{128} &  21,399,552 &           20.42 ± 8.39 &           -8.33 ± 1.73 &            0.00 ± 0.00 &           0.00 ± 0.00 \\
    &    & \textbf{256} &  42,633,216 &            5.31 ± 6.63 &          -10.61 ± 0.95 &            0.00 ± 0.00 &           0.00 ± 0.00 \\
\cline{1-8}
\cline{2-8}
\multirow{3}{*}{\textbf{NCA}} & \multirow{3}{*}{\textbf{16}} & \textbf{96 } &      84,672 &           45.85 ± 2.83 &           79.20 ± 0.83 &           31.44 ± 1.26 &           2.69 ± 2.23 \\
    &    & \textbf{128} &     149,760 &           69.98 ± 1.62 &  \textbf{79.75} ± 0.40 &           39.42 ± 0.95 &           2.82 ± 2.16 \\
    &    & \textbf{256} &     594,432 &  \textbf{96.80} ± 0.65 &           79.13 ± 0.54 &  \textbf{49.76} ± 1.16 &  \textbf{5.47} ± 2.12 \\
\hline
\end{tabular}
