# Supplementary material for: Pathfinding Neural Cellular Automata
Source: arXiv:2301.06820 source file (2023-01-17)
Supplement: Supplementary file 7 [file pathfinding_cut_corners_cross_eval_selective.tex]

\begin{tabular}{|c|r|r|r|r|r|r|r|}
\hline
    &      &    &      model &                  train & \multicolumn{3}{c|}{test} \\
\cline{4-8}
\cline{4-8}
    &      &    &        --- &                  16x16 &                  16x16 & \multicolumn{2}{c|}{32x32} \\
\cline{4-8}
\cline{4-8}
    &      &    &  n. params &          pct. complete &          pct. complete &             accuracies &          pct. complete \\
\textbf{model} & \textbf{cut corners} & \textbf{n. hid chan} &            &                        &                        &                        &                        \\
\hline
\multirow{4}{*}{\textbf{NCA}} & \multirow{2}{*}{\textbf{False}} & \textbf{48} &  1,437,696 &  \textbf{99.93} ± 0.05 &           94.82 ± 0.52 &           79.65 ± 1.46 &           80.83 ± 4.11 \\
    &      & \textbf{96} &  5,529,600 &           99.84 ± 0.10 &  \textbf{95.90} ± 0.55 &  \textbf{81.82} ± 3.11 &  \textbf{84.59} ± 1.35 \\
\cline{2-8}
    & \multirow{2}{*}{\textbf{True}} & \textbf{48} &    798,720 &           99.69 ± 0.35 &           94.45 ± 1.01 &          64.10 ± 15.54 &          65.47 ± 10.81 \\
    &      & \textbf{96} &  3,072,000 &          79.86 ± 44.64 &          76.44 ± 42.73 &          64.21 ± 35.97 &          64.91 ± 36.44 \\
\hline
\end{tabular}
