# Supplementary material for: Pathfinding Neural Cellular Automata
Source: arXiv:2301.06820 source file (2023-01-17)
Supplement: Supplementary file 8 [file pathfinding_evo_data_cross_eval_selective.tex]

\begin{tabular}{|c|r|r|r|r|r|r|r|r|}
\hline
    &       &     &     model & \multicolumn{2}{c|}{train} & \multicolumn{3}{c|}{test} \\
\cline{4-9}
\cline{4-9}
    &       &     &       --- & \multicolumn{2}{c|}{16x16} & \multicolumn{2}{c|}{16x16} &                  32x32 \\
\cline{4-9}
\cline{4-9}
    &       &     & n. params &                sol len &          pct. complete &             accuracies &          pct. complete &             accuracies \\
\textbf{model} & \textbf{env generation} & \textbf{n. hid chan} &           &                        &                        &                        &                        &                        \\
\hline
\multirow{4}{*}{\textbf{NCA}} & \multirow{2}{*}{\textbf{False}} & \textbf{96 } &    86,400 &            9.02 ± 0.00 &          78.53 ± 43.92 &          77.09 ± 43.10 &          76.84 ± 42.97 &          65.99 ± 37.70 \\
    &       & \textbf{128} &   152,064 &            9.02 ± 0.00 &  \textbf{99.37} ± 0.24 &           97.44 ± 0.13 &           97.61 ± 0.20 &           90.06 ± 2.93 \\
\cline{2-9}
    & \multirow{2}{*}{\textbf{True }} & \textbf{96 } &    86,400 &           21.39 ± 6.99 &          74.06 ± 41.44 &          79.18 ± 44.26 &          79.21 ± 44.28 &          78.12 ± 43.67 \\
    &       & \textbf{128} &   152,064 &  \textbf{23.75} ± 1.36 &           92.92 ± 3.79 &  \textbf{98.88} ± 0.36 &  \textbf{99.34} ± 0.11 &  \textbf{97.17} ± 2.15 \\
\hline
\end{tabular}
