# Supplementary material for: Pathfinding Neural Cellular Automata
Source: arXiv:2301.06820 source file (2023-01-17)
Supplement: Supplementary file 9 [file pathfinding_kernel_cross_eval_selective.tex]

\begin{tabular}{|c|r|r|r|r|r|r|r|r|}
\hline
    &   &       &    &       model &                  train & \multicolumn{3}{c|}{test} \\
\cline{5-9}
\cline{5-9}
    &   &       &    &         --- &                  16x16 &                  16x16 & \multicolumn{2}{c|}{32x32} \\
\cline{5-9}
\cline{5-9}
    &   &       &    &   n. params &          pct. complete &          pct. complete &             accuracies &          pct. complete \\
\textbf{model} & \textbf{kernel size} & \textbf{max pool} & \textbf{n. hid chan} &             &                        &                        &                        &                        \\
\hline
\multirow{4}{*}{\textbf{NCA}} & \multirow{2}{*}{\textbf{3}} & \multirow{2}{*}{\textbf{False}} & \textbf{48} &   1,437,696 &  \textbf{99.93} ± 0.05 &           94.82 ± 0.52 &           79.65 ± 1.46 &           80.83 ± 4.11 \\
    &   &       & \textbf{96} &   5,529,600 &           99.84 ± 0.10 &  \textbf{95.90} ± 0.55 &  \textbf{81.82} ± 3.11 &  \textbf{84.59} ± 1.35 \\
\cline{2-9}
\cline{3-9}
    & \multirow{2}{*}{\textbf{5}} & \multirow{2}{*}{\textbf{False}} & \textbf{48} &   3,993,600 &           99.87 ± 0.07 &           92.37 ± 1.08 &           72.86 ± 2.35 &           79.28 ± 1.90 \\
    &   &       & \textbf{96} &  15,360,000 &           99.86 ± 0.07 &           92.37 ± 0.78 &           75.51 ± 2.17 &           79.92 ± 2.11 \\
\hline
\end{tabular}
