# Supplementary material for: Pathfinding Neural Cellular Automata
Source: arXiv:2301.06820 source file (2023-01-17)
Supplement: Supplementary file 10 [file pathfinding_max_pool_cross_eval_selective.tex]

\begin{tabular}{|c|r|r|r|r|r|r|r|}
\hline
    &      &     &      model &                  train & \multicolumn{3}{c|}{test} \\
\cline{4-8}
\cline{4-8}
    &      &     &        --- &                  16x16 &                  16x16 & \multicolumn{2}{c|}{32x32} \\
\cline{4-8}
\cline{4-8}
    &      &     &  n. params &          pct. complete &          pct. complete &             accuracies &          pct. complete \\
\textbf{model} & \textbf{max pool} & \textbf{n. hid chan} &            &                        &                        &                        &                        \\
\hline
\multirow{6}{*}{\textbf{NCA}} & \multirow{3}{*}{\textbf{False}} & \textbf{48 } &  1,437,696 &  \textbf{99.93} ± 0.05 &           94.82 ± 0.52 &           79.65 ± 1.46 &           80.83 ± 4.11 \\
    &      & \textbf{96 } &  5,529,600 &           99.84 ± 0.10 &           95.90 ± 0.55 &           81.82 ± 3.11 &           84.59 ± 1.35 \\
    &      & \textbf{128} &  9,732,096 &           99.87 ± 0.06 &           95.78 ± 0.71 &           80.68 ± 2.41 &           85.14 ± 2.01 \\
\cline{2-8}
    & \multirow{3}{*}{\textbf{True}} & \textbf{48 } &  1,437,696 &           99.69 ± 0.25 &           93.51 ± 0.81 &           77.02 ± 2.34 &           79.45 ± 2.91 \\
    &      & \textbf{96 } &  5,529,600 &           99.85 ± 0.09 &           95.83 ± 0.40 &           83.10 ± 2.79 &           84.69 ± 2.69 \\
    &      & \textbf{128} &  9,732,096 &           99.87 ± 0.02 &  \textbf{96.48} ± 0.45 &  \textbf{85.96} ± 2.35 &  \textbf{85.57} ± 2.42 \\
\hline
\end{tabular}
