# Supplementary material for: Pathfinding Neural Cellular Automata
Source: arXiv:2301.06820 source file (2023-01-17)
Supplement: Supplementary file 11 [file pathfinding_max_pool_cross_eval_selective_many1.tex]

\begin{tabular}{|c|r|r|r|r|r|r|r|}
\hline
    &      &     &     model &                  train & \multicolumn{3}{c|}{test} \\
\cline{4-8}
\cline{4-8}
    &      &     &       --- &                  16x16 &                  16x16 & \multicolumn{2}{c|}{32x32} \\
\cline{4-8}
\cline{4-8}
    &      &     & n. params &          pct. complete &          pct. complete &             accuracies &          pct. complete \\
\textbf{model} & \textbf{max pool} & \textbf{n. hid chan} &           &                        &                        &                        &                        \\
\hline
\multirow{10}{*}{\textbf{NCA}} & \multirow{5}{*}{\textbf{False}} & \textbf{48 } &    22,464 &           98.43 ± 1.58 &           96.53 ± 2.37 &           88.98 ± 5.41 &           90.08 ± 3.45 \\
    &      & \textbf{64 } &    39,168 &           97.47 ± 1.81 &           95.18 ± 2.66 &          49.48 ± 13.98 &           71.51 ± 5.91 \\
    &      & \textbf{96 } &    86,496 &           99.12 ± 1.17 &           97.55 ± 2.02 &           87.37 ± 6.07 &           90.25 ± 3.46 \\
    &      & \textbf{128} &   152,064 &           98.90 ± 1.33 &           97.63 ± 1.88 &           91.72 ± 4.85 &           92.75 ± 3.38 \\
    &      & \textbf{150} &   207,900 &           99.06 ± 1.11 &           97.86 ± 1.86 &  \textbf{93.73} ± 3.67 &           93.91 ± 2.51 \\
\cline{2-8}
    & \multirow{5}{*}{\textbf{True}} & \textbf{48 } &    22,464 &           98.50 ± 1.60 &           96.22 ± 2.23 &           87.79 ± 6.44 &           91.30 ± 3.63 \\
    &      & \textbf{64 } &    39,168 &           99.05 ± 1.11 &           96.66 ± 2.15 &           84.52 ± 6.66 &           88.37 ± 3.74 \\
    &      & \textbf{96 } &    86,400 &           98.43 ± 1.44 &           96.58 ± 2.41 &           86.52 ± 6.33 &           89.33 ± 3.95 \\
    &      & \textbf{128} &   152,064 &           99.24 ± 1.10 &           98.02 ± 1.78 &           92.65 ± 4.26 &  \textbf{93.99} ± 2.88 \\
    &      & \textbf{150} &   207,900 &  \textbf{99.40} ± 0.96 &  \textbf{98.27} ± 1.59 &           89.79 ± 5.34 &           92.87 ± 3.13 \\
\hline
\end{tabular}
