# Supplementary material for: Pathfinding Neural Cellular Automata
Source: arXiv:2301.06820 source file (2023-01-17)
Supplement: Supplementary file 12 [file pathfinding_models_cross_eval_selective.tex]

\begin{tabular}{|c|r|r|r|r|r|r|r|}
\hline
    &    &     &       model &                  train & \multicolumn{3}{c|}{test} \\
\cline{4-8}
\cline{4-8}
    &    &     &         --- &                  16x16 & \multicolumn{2}{c|}{16x16} &                  32x32 \\
\cline{4-8}
\cline{4-8}
    &    &     &   n. params &          pct. complete &             accuracies &          pct. complete &          pct. complete \\
\textbf{model} & \textbf{n layers} & \textbf{n. hid chan} &             &                        &                        &                        &                        \\
\hline
\multirow{3}{*}{\textbf{GCN}} & \multirow{3}{*}{\textbf{16}} & \textbf{96 } &       9,600 &           11.51 ± 1.47 &           31.59 ± 1.08 &           12.29 ± 1.52 &            0.21 ± 0.10 \\
    &    & \textbf{128} &      16,896 &           11.58 ± 6.72 &          26.98 ± 15.10 &           11.87 ± 6.83 &            0.07 ± 0.06 \\
    &    & \textbf{256} &      66,560 &          11.96 ± 10.92 &          22.34 ± 20.37 &          11.75 ± 10.73 &            0.21 ± 0.26 \\
\cline{1-8}
\cline{2-8}
\multirow{3}{*}{\textbf{MLP}} & \multirow{3}{*}{\textbf{16}} & \textbf{96 } &  16,257,024 &           36.07 ± 3.12 &           12.64 ± 1.41 &            2.62 ± 0.19 &            0.00 ± 0.00 \\
    &    & \textbf{128} &  21,565,440 &           36.84 ± 3.60 &           11.69 ± 1.51 &            2.26 ± 0.24 &            0.00 ± 0.00 \\
    &    & \textbf{256} &  42,799,104 &           21.15 ± 8.83 &            6.71 ± 1.27 &            2.08 ± 0.38 &            0.00 ± 0.00 \\
\cline{1-8}
\cline{2-8}
\multirow{3}{*}{\textbf{NCA}} & \multirow{3}{*}{\textbf{16}} & \textbf{96 } &      86,400 &           99.82 ± 0.15 &           95.38 ± 0.55 &           93.07 ± 0.60 &          70.40 ± 35.18 \\
    &    & \textbf{128} &     152,064 &           99.93 ± 0.06 &           95.90 ± 0.56 &           94.02 ± 0.66 &          61.37 ± 32.02 \\
    &    & \textbf{256} &     599,040 &  \textbf{99.94} ± 0.05 &  \textbf{96.80} ± 0.36 &  \textbf{96.09} ± 0.38 &  \textbf{90.00} ± 0.52 \\
\hline
\end{tabular}
